# Supplementary material for: Structuro-elasto-plasticity (StEP) model for plasticity in disordered solids
Source: arXiv:2205.08678 source file (2022-05-18)
Supplement: Supplementary file 1 [file supplementary.pdf]

# Supplementary information for structuro-elasto-plasticity (StEP) model for plasticity in disordered solids


Ge Zhang,[1] Hongyi Xiao,[2] Entao Yang,[3] Robert J. S. Ivancic,[4] Sean A. Ridout,[2] Robert Riggleman,[3] Douglas J. Durian,[2] and Andrea J. Liu[2,*]

[1]Department of Physics, City University of Hong Kong, *Hong Kong, China*

[2]Department of Physics and Astronomy, University of Pennsylvania, *Philadelphia PA 19104*

[3]Department of Chemical and Biomolecular Engineering, University of Pennsylvania, *Philadelphia PA 19104*

[4]Materials Science and Engineering Division, National Institute of Standards and Technology, *Gaithersburg, MD 20899*


## I. IDENTIFYING REARRANGEMENTS IN PARTICLE SIMULATIONS

We calculate the nonaffine displacement of each particle $n$ [1]: $D^2_{\text{min}} = \left\langle \left(\mathbf{r}'_n - \mathbf{J}\mathbf{r}_n\right)^2 \right\rangle$, where $\langle \cdots \rangle$ indicates an average over all neighbor particles within a distance of $R_D = 2$, $\mathbf{r}_n$ and $\mathbf{r}'_n$ are the vector separations between particle $n$ and neighbor $n'$ during a period where the root mean squared total displacement, $\sqrt{\sum_i^N \delta\mathbf{r}_i^2}$, is 0.15. $\mathbf{J}$ is the "best-fit" local deformation gradient tensor that minimizes $D^2_{\text{min}}$. A small/large particle "rearranges" if $D^2_{\text{min}} > 0.0025/D^2_{\text{min}} > 0.0015$.

## II. INSTANTANEOUS $D^2_{\text{min}}$ CORRELATION FUNCTION

One component of our model is the spatial scale of a rearrangement. To measure that from the particle simulations, we calculated the $D^2_{\text{min}}$ correlation function using the shortest possible time scale (corresponding to a strain of $10^{-5}$), shown in Fig. S1. As shown in the supplementary movie of Ref. 2, most of these frames contain zero or one rearrangement event. Thus, this $D^2_{\text{min}}$ correlation function measures the size of a single rearrangement, rather than the spatial correlation of multiple rearrangement events.


* ajliu@physics.upenn.edu

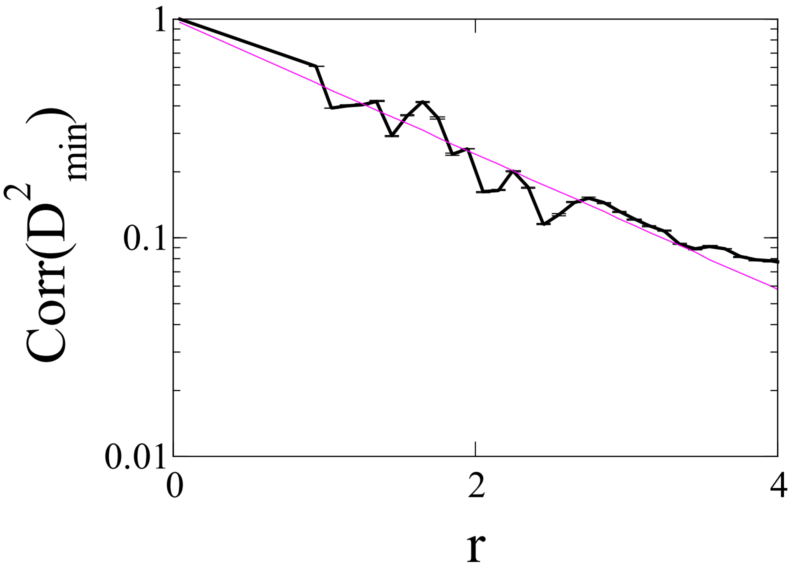


FIG. S1. The Pearson correlation function of $D^2_{\text{min}}$ at two points with a distance of $r$ in our particle simulation. Magenta line is the fit $\text{Corr}(D^2_{\text{min}}) = \exp(-r/1.40179)$.

### III. STRAIN RELEASE PER FRAME IN PARTICLE SIMULATIONS

In particle simulations described in Ref. 2, where we studied the evolution during stress drops, we recorded a frame when the sum of particle displacement squared reached a threshold. Here we show multiple pieces of evidence that this approach leads to a deviatoric strain release of about $\epsilon = 0.1$ per unit volume per frame. The measured $\epsilon$ is used as a parameter in our StEP model, to make fair comparison of the StEP model predictions with particle simulations for the pair correlation function of rearrangers [Fig. 3(c) of the main text].

First we calculate the locally-extracted deformation tensor. Within a distance of $R_D$ from a rearranger, we perform a local fit to find the local affine deformation tensor $J$, and extract a deviatoric strain $\varepsilon_f$ from $J$, as detailed in Ref. 2. As shown in Fig. S2, the fitting area times $\varepsilon_f$ approaches about 0.1 as the fitting range increases.

Second, we found earlier that the deviatoric strain field per frame caused by a rearranger is well-fit by the function $\tilde{\epsilon}(r) = 0.03r^{-2}$ in the particle simulations, see Fig. 3 of Ref. 2. In our StEP model, each block has a side length of 1, so for the rearranging block, the distance between its center and one of its edge is about $r = 0.5$. Thus the strain field at the edge of

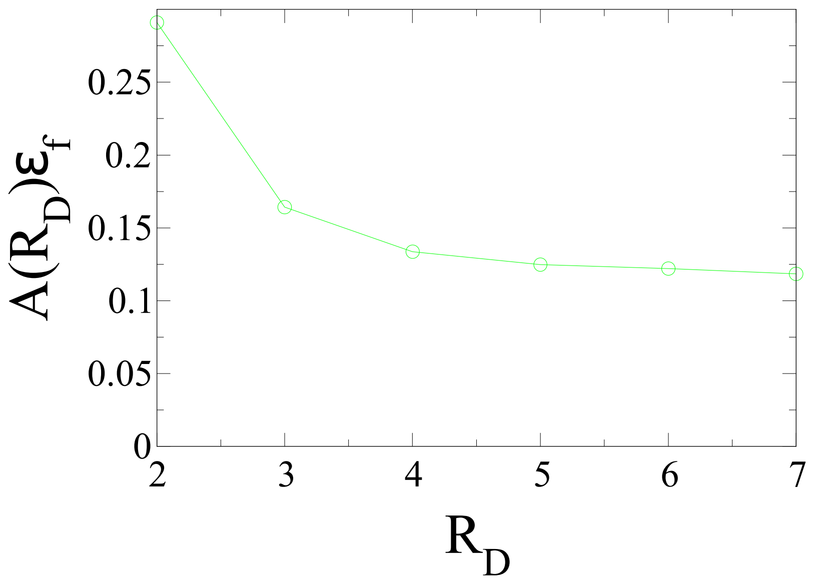


FIG. S2. The fitted deviatoric strain $\varepsilon_f$ times the area of the fitted region $A(R_D) = \pi R_D^2$ versus the fitting radius $R_D$.

the block is $\tilde{\epsilon}(r = 0.5) \approx 0.1$.

Finally, we collected $N_f = 7.2{\times}10^5$ frames per unit global strain in our particle simulation. Most of these frames contain a single rearrangement. Since we have a total of $N = 10^5$ particles, and since the global strain is imposed upon each particle, the strain release per frame is roughly $N/N_f \approx 0.1$.

## IV. DETAILED BALANCE ARGUMENT FOR NOISE TERM

The softness change due to rearrangements in our model is captured by the sum of three terms: a restoring term, an angular term, and a noise term. We plan to use this model to study thermal systems in the future, thus we also incorporate constraints to satisfy detailed balance. The restoring term and noise term can be correlated in the spirit of detailed balance, because rearrangements should not lead to change in average softness when the system is in equilibrium. Due to the existence of angular term, we assume detailed balance is satisfied at each distance from the rearranger.

Our numerical measurements suggest that: 1) system softness follows a Gaussian dis-

tribution, with a constant mean, $\mu$, and variance, $\sigma^2$, during shearing ($P(S) \propto \mathcal{N}(\mu, \sigma^2)$); 2) the probability that a particle will rearrange increases exponentially with its softness ($P(R|S) \propto e^{\gamma S}$); 3) the mean softness change of a particle at a distance $r$ from a rearranger, $\mu_R(r)$, is a linear function of the particle's current softness:

$$\mu_R(r) = \eta(r) \times (S_0(r) - S) \tag{1}$$

This is the restoring term, where the prefactor $\eta(r)$ decays with distance $r$, and $S_0(r)$. We will show later that $S_0(r)$ is the average softness at r, if we assume the distribution of softness change in every step is also Gaussian:

$$P(\Delta S_R) \propto \mathcal{N}(\mu_R, \sigma_R^2) \tag{2}$$

We start our derivation from rearranging particles. Since detailed balance is satisfied at different distances to the rearrangers respectively, rearranging particles ($r = 0$) themselves satisfy detailed balance:

$$\begin{aligned} &P(S_1) \cdot P(R|S_1) \cdot G(S_1, S_2) \\ &= P(S_2) \cdot P(R|S_2) \cdot G(S_2, S_1) \end{aligned} \tag{3}$$

where $P(S)$ is particle's probability of having softness $S$, $P(R|S_1)$ is particle's rearranging probability when it has softness $S$, $G(S_1, S_2)$ is the transition probability that softness change from $S_1$ to $S_2$ after one step. By definition above, we can write the expression of $G(S_1, S_2)$:

$$G(S_1, S_2) \propto \exp\left(-\frac{(S_2 - S_1) - \mu_R^2}{2\sigma_R^2}\right) \tag{4}$$

where $\mu_R = \eta(r)(S_0(r) - S)$. Substituting it back to the detailed balance equation, we can finally see that softness of rearranging particles also follows a normal distribution:

$$P(S|R) \propto \mathcal{N}(S_0, \frac{\sigma_R^2}{\eta(2-\eta)}) \tag{5}$$

From Eqn.(5) above, we know that $S_0$ is the average softness of rearranging particles. To solve for $\sigma_R^2$, we can employ Bayes theorem:

$$P(S|R) = \frac{P(R|S) \cdot P(S)}{P(R)} \tag{6}$$

For a given system at a certain step, the overall rearranging probability, $P(R)$, is a constant. $P(R|S)$ increases exponentially with softness. Thus,

$$\begin{aligned} P(S|R) &\propto P(R|S) \cdot P(S) \propto \exp\{\gamma S\} \cdot \exp\left\{-\frac{(S-\mu)^2}{2\sigma^2}\right\} \\ &\propto \exp\left(-\frac{(S - (\mu + \gamma\sigma^2))^2}{2\sigma^2}\right) \end{aligned} \tag{7}$$

Here, we get a new expression for the softness distribution of rearranging particles, $P(S|R) \propto \mathcal{N}(\mu + \gamma\sigma^2, \sigma^2)$. This leads to the first conclusion we can draw from detailed balance:

$$\frac{\sigma_R(0)^2}{\eta(0) \cdot (2 - \eta(0))} = \sigma^2 \tag{8}$$

The standard deviation, $\sigma_R$, of softness change for rearrangers is correlated with $\eta$. For non-rearranging particles, the detailed balance equation is different:

$$P(S_1|r = r_0) \cdot G(S_1, S_2) = P(S_2|r = r_0) \cdot G(S_2, S_1) \tag{9}$$

where $P(S_1|r = r_0)$ is the probability that we see softness $S_1$ at $r = r_0$. Similar as rearranging particles, we can arrive at a new expression of $P(S|r = r_0)$ by substituting all terms:

$$P(S|r_0) \propto \exp\left(-\frac{(\eta(r_0)(2 - \eta(r_0))}{2\sigma_R^2(r_0)}(S_0(r_0) - S)^2\right) \tag{10}$$

By definition of $P(S|r_0)$, we know that $S_0(r_0)$ should be the angular average softness at $r = r_0$ (same for the the variance). This leads to the second conclusion we can draw from detailed balance:

$$S_0(r) =< S(r) > \tag{11}$$

$$\frac{\sigma_R(r)^2}{\eta(r) \cdot (2 - \eta(r))} = \sigma^2 \tag{12}$$

## V. AVALANCHE-SIZE DISTRIBUTION SCALING EXPONENTS

Here we present avalanche-size distributions of the StEP model for five different system sizes, and measure the scaling exponents. As shown in Fig. S3, the distributions for different system sizes collapse well using the exponents reported in the main text.

---


[1] M. L. Falk and J. S. Langer, Dynamics of viscoplastic deformation in amorphous solids, Phys. Rev. E **57**, 7192 (1998).

[2] G. Zhang, S. A. Ridout, and A. J. Liu, Interplay of rearrangements, strain, and local structure during avalanche propagation, Phys. Rev. X **11**, 041019 (2021).

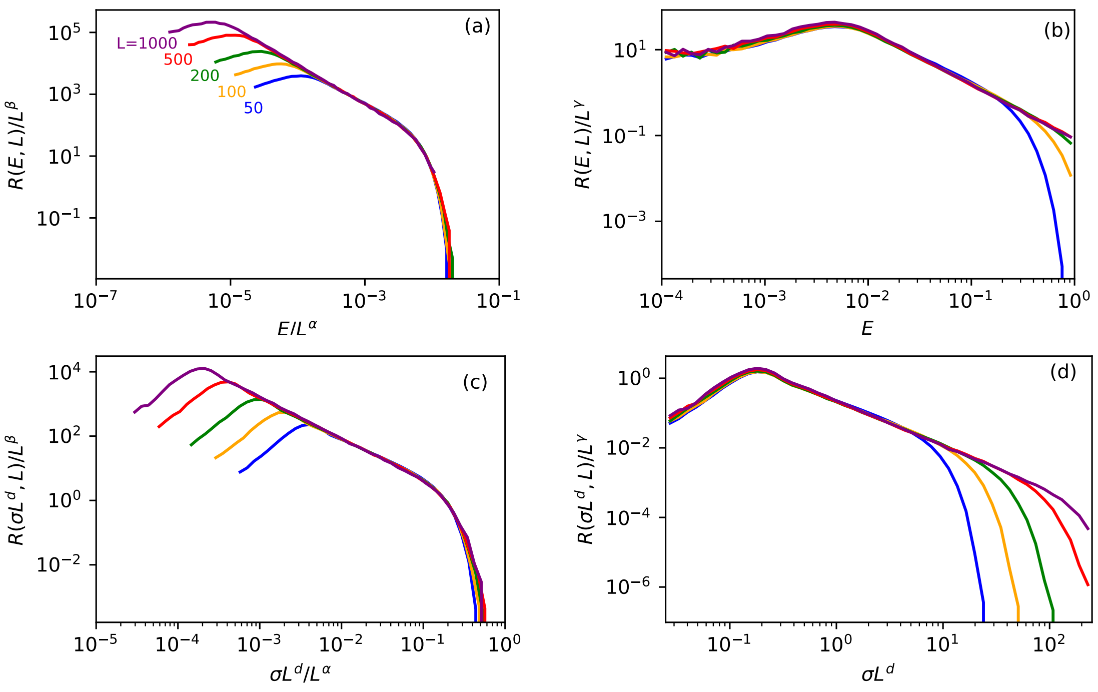


FIG. S3. Finite-size scaling collapse of energy-drop rate $R(E, L)$ for the StEP model. The curves for different system sizes align well with exponents reported in the main text. (bottom) Same as top, except for the rate of the rescaled stress drop $\sigma L^d$, where $d = 2$ is the space dimension.
